# Supplementary material for: Understanding the Power of Evolutionary Computation for GPU Code Optimization
Source: arXiv:2208.12350 source file (2022-08-25)
Supplement: Supplementary file 1 [file appendix.tex]

\section{Analyzing Fine-Grained, Low-Level Edits in the Context of the Original Source Code}
\label{sec:edit_alyz}
In this section, we take a deeper dive into understanding the functional impact on the runtime performance of remaining code edits from Section~\ref{sec:edit_characteristic}, by tracing the code edit in LLVM-IR back to the corresponding source code implementation in the high-level programming language, i.e., CUDA for this paper. While requiring significant manual efforts, this is an important attempt to understand performance optimization opportunities that evolutionary code transformation approaches can uncover. 

\definecolor{backcolour}{rgb}{0.95,0.95,0.92}
\definecolor{codegreen}{rgb}{0,0.6,0}
\definecolor{codegray}{rgb}{0.5,0.5,0.5}
\definecolor{codepurple}{rgb}{0.58,0,0.82}
\definecolor{backcolour}{rgb}{0.95,0.95,0.92}

\begin{figure}
\lstdefinestyle{mystyle}{
    language=C++,
    morekeywords = {__shared__, __syncthreads, __shfl_sync},
    otherkeywords = {__shared__, __syncthreads, __shfl_sync},
    backgroundcolor=\color{backcolour},
    keywordstyle=\bfseries\color{blue},
    numberstyle=\ttfamily\small\color{codegray},
    commentstyle=\color{codegreen},
    basicstyle=\footnotesize\ttfamily,
    numbers=left,
    frame=single,framexleftmargin=3em,
    stepnumber=1,
    showstringspaces=false,
    tabsize=1,
    breaklines=true,
    breakatwhitespace=false,
    xleftmargin=8.0ex,
    moredelim=[is][\bfseries\color{red}]{<<<}{>>>},
}
\lstset{style=mystyle}
\begin{lstlisting}
int tID = threadIdx.x;
short warpId = tID/32;
short landID = tid%32;
__shared__ short sh_prev_E[32]; 
__shared__ short sh_prev_H[32];
__shared__ short sh_prev_prev_H[32];
__shared__ short local_prev_E[1024];
__shared__ short local_prev_H[1024];
__shared__ short local_prev_prev_H[1024];
...
// if (laneId == 31)
<<<if (landId == 0) { >>>// edit 5 
  sh_prev_E[warpId] = _prev_E;
  sh_prev_H[warpId] = _prev_H;
  sh_prev_prev_H[warpId] = _prev_prev_H;
}

// if(diag >= maxSize)
<<<if (tID < minSize) { >>>// edit 6
  local_prev_E[tID] = _prev_E;
  local_prev_H[tID] = _prev_H;
  local_prev_prev_H[tID] = _prev_prev_H;
}

__syncthreads();

if (is_valid[tID] && tID < minSize) {
  ...
  // if(diag >= maxSize) {
  <<<if (is_valid[tID]) { >>> // edit 8
    eVal = local_prev_E[tID-1] + extendGap;
    heVal = local_prev_H[tID-1] + startGap;
  }
  else {
    if (warpId != 0 && landId == 0) {
      eVal = sh_prev_E[warpId-1];
      heVal = sh_prev_H[warpId-1];
    } else { // private register
      eVal = __shfl_sync(...); 
      heval = __shfl_sync(...);
    }
  }
  
  // if(diag >= maxSize) {
  <<<if (is_valid[tID]) { >>> // edit 10
    final_H = local_prev_prev_H[tID-1];
  }
  else {
    if (warpId != 0 && landId == 0) {
      final_H = sh_prev_prev_H[warpId-1];
    } else { // private register
      final_H = __shfl_sync(...); 
    }
  }
  ...
}
...

\end{lstlisting}
\caption{Simplified code snippet from ADEPT for how data is exchanged using both private registers and shared memory. The 4 edits (edit 5, 6, 8, and 10), made by GEVO are highlighted in red color in lines 12, 19, 30, and 45, where GEVO eliminates private registers usage and uses the shared memory completely instead.}
\label{fig:data_exchange}
\end{figure}

\subsection{Rearrange the usage of sub-memory systems on GPU}

GEVO alters how ADEPT-o utilizes GPU's sub-memory systems, the shared memory and private registers -- through the same epistatic edits discussed in Section~\ref{sec:epistasis_alyz}. By doing so, GEVO achieves 15\% performance improvement on the P100 GPU. These edits are applicable on the V100 GPU as well, achieving similar performance improvement. Recall that, in Section~\ref{sec:ADEPT}, ADEPT-o uses both private registers and shared memory to exchange data. Its implementation is shown in Figure~\ref{fig:data_exchange}, where the edits are marked in red text. These edits essentially eliminate the use of private registers and rely on the shared memory only. 

The $else$ clause around lines 38-41 and 51-53 are for the thread that meets the conditions to share data through private registers using the $shfl\_sync$ function. Due to the limitation of the GPU architecture, the threads that cannot exchange data through private registers will go through shared memory. The goal of edits 8 (line 30) and 10 (line 45) is to drop the use of the private register. It is achieved by replacing the corresponding $if$ condition using the existing boolean expression from line 27. If the boolean expression in line 27 is true, both lines 30 and 45 will be evaluated as true. This effectively makes every relevant thread in the code snippet write/read the data to/from the shared memory regardless of any other condition. However, edits 8 and 10 cannot be applied alone without edit 6 that implicitly enables every thread writing their data to the shared memory named \textit{local\_prev\_XX}.  After applying the above 3 edits, the shared memory named \textit{sh\_prev\_XX} is no longer needed, leading to edit 5. A human developer often at this stage would remove the entire $if$ clause in lines 11-16 since the shared memory within the if clause is not referred to anymore. Instead of removing the shared memory, GEVO introduces edit 5 that only changes which thread will access that shared memory. However, this modification has the same performance improvement as the affected code snippet was removed. We assume, by changing the memory access pattern as edit 5 does, the GPU can schedule the memory access differently and hide the memory latency of this particular access.

Accessing private registers on GPUs is much faster than the shared memory. So then, how do edits prefer shared memory achieve performance advantage? This might be related to the branch divergence. From Section~\ref{sec:ADEPT} and Figure~\ref{fig:adept-parallel}, while some threads in a warp can utilize private registers for data sharing, there must be one thread, usually the first thread in the warp, that must communicate through the shared memory. Combining with the GPU lock-step execution model (Every thread in the same warp executes the same instruction at the same time), the above behavior guarantees the branch divergence in the if-else region between lines 35-41 and 49-53. This essentially forces every thread in the same warp to run through both if and else regions, and whichever thread uses private registers has to wait for the slowest thread that accesses the shared memory to finish. As a result, this behavior eliminates the advantage of the fast access speed from the private register.

\begin{figure}[t]
\lstdefinestyle{mystyle}{
    language=C++,
    morekeywords = {__shared__},
    otherkeywords = {__shared__},
    backgroundcolor=\color{backcolour},
    keywordstyle=\bfseries\color{blue},
    numberstyle=\ttfamily\small\color{codegray},
    commentstyle=\color{codegreen},
    basicstyle=\footnotesize\ttfamily,
    numbers=left,
    frame=single,framexleftmargin=3em,
    stepnumber=1,
    showstringspaces=false,
    tabsize=1,
    breaklines=true,
    breakatwhitespace=false,
    xleftmargin=8.0ex,
    moredelim=[is][\bfseries\color{red}]{<<<}{>>>},
}
\lstset{
  style=mystyle,
  moredelim=[is][\bfseries\color{red}]{<<<}{>>>},
  moredelim=[is][\sout]{|}{|}
}
\begin{lstlisting}
int tID = threadIdx.x;
__shared__ char curr_H, curr_E, curr_F;
...
|__syncthreads();| // edit 1
for (...){
  curr_H = ...
  |memset(curr_H, 0, size);| // edit 2
  |__syncthreads();| // edit 3
  
  curr_F = ...
  |memset(curr_F, 0, size);| // edit 4
  |__syncthreads();| // edit 5
  
  curr_E = ...
  |memset(curr_E, 0, size);| // edit 6
  |__syncthreads();| // edit 7
  
  if(is_valid[tID] && tID < minSize) {
    ... // calculate the scoring matrix
  }
}


\end{lstlisting}
\caption{Edits remove unnecessary memory initialization and synchronization operations. They are found in ADEPT-b and applicable for all GPUs.}
\label{fig:meminit}
\end{figure}

\subsection{Remove warp-level synchronization}
The CUDA programming guide suggests that, before exchanging the data through the private register, the programmer should invoke the query function, such as \textit{activemask} or \textit{ballot\_sync}, to return a mask indicating which threads are still alive in the warp. In particular, after the NVIDIA Volta GPU architecture (V100 GPU in our testing environment), \textit{ballot\_sync} should be used as the query function inside any conditional branch where branch divergence can happen. This is because Volta architecture allows GPU to further divide a warp into subgroups to be scheduled independently, and \textit{ballot\_sync} implicitly forces GPU to synchronize threads in the same warp. 

Perhaps to be conservative, the developers of ADEPT use both \textit{activemask} and \textit{ballot\_sync} before accessing the private registers in a conditional branch. An independent edit shows that removing \textit{ballot\_sync} can yield 4\% performance improvement on the V100 GPU but not on the P100 GPU, which verifies that \textit{ballot\_sync} does perform warp-level synchronization on the Volta GPU architecture but not on older GPU generations. 
This edit is interesting because it actually violates what the CUDA programming guide suggests~\cite{warplevelprimitives}!
Despite the violation, the edit still passes all the verification tests. However, due to the proprietary design of the Volta GPU warp scheduler, we cannot conclude in what situations removing warp-level synchronization is safe. 

\subsection{Remove unnecessary memory initialization and synchronization}
We describe another performance optimization opportunity GEVO found by an epistasis consisting of seven edits on ADEPT-b. As depicted in Figure~\ref{fig:meminit}, this epistasis improves the kernel performance of ADEPT-b by more than 30 times. It is impressive such tremendous performance improvement can be achieved with only a few edits.

It appears that we can completely ignore shared memory initialization, i.e., skipping \textit{memset} in lines 7, 11, and 15 in Figure~\ref{fig:meminit}, even on the algorithm level. This is because GEVO does not engage other edits to compensate for the behavior change. They are indeed removed in the ADEPT-o, the version of ADEPT that was further optimized by the developers. Even though such initialization is required, the way it is implemented is vastly inefficient. The original code asks all the GPU threads to perform memory initialization on the same memory region. Combined with synchronization (\textit{syncthread} in lines 8, 12, and 16), GPU threads block each other to initialize the same memory region over and over again, leading to a huge performance bottleneck. The common practice is to initialize the memory through the CUDA API outside the kernel or through the in-kernel code  with only one active thread.
We note that the last synchronization primitive (line 16 in Figure~\ref{fig:meminit}) cannot be removed until all \textit{memset} functions are removed first, or a race condition will arise. Thus, these edits are epistatic due to this dependency.

\subsection{Others}
While we do our best to analyze all the edits we can, there are some edits that we are unable to reason about. For example, one edit duplicates a memory write operation to a region that no subsequent code will ever access. Such seemingly redundant operation, instead of slowing down the program, surprisingly improves the performance by 1\%, though only on the P100 GPU.
